# Supplementary material for: Convergence of Heavy-Flavor PDFs at Small x and Its Impact on Future ep Colliders
Source: arXiv:2510.15427 source file (2026-01-20)
Supplement: Supplementary file 1 [file supplemental.pdf]

# Supplemental Material for *Convergence of Heavy-Flavor PDFs at Small $x$ and Its Impact on Future $ep$ Colliders*

S. O. Kara<sup>1</sup>

<sup>1</sup>*Niğde Ömer Halisdemir University, Bor Vocational School, 51240 Niğde, Türkiye*

**Published in:** Physical Review Letters (submitted).

**Corresponding author:** seyitokankara@gmail.com

**This Supplemental Material** provides the complete mathematical definitions, numerical setup, and stability tests underlying the results reported in the main Letter. All notation and conventions follow those introduced therein. The data grids used for the Mahalanobis and Kullback–Leibler analyses are available as ancillary files.

## A. STATISTICAL DEFINITIONS

Detailed expressions for the Mahalanobis tension and the Kullback–Leibler (KL) divergence used in the main text are summarized below. For any two PDF ensembles  $i$  and  $j$ , the global tension reads

$$T_{\text{PDF}}^2(i, j) = (\boldsymbol{\mu}_i - \boldsymbol{\mu}_j)^\top \boldsymbol{\Sigma}^{-1} (\boldsymbol{\mu}_i - \boldsymbol{\mu}_j), \quad (1)$$

where  $\boldsymbol{\mu}_k \equiv \langle f \rangle_k$  is the mean observable vector and  $\boldsymbol{\Sigma}$  is the combined covariance matrix. For statistically independent fits,  $\boldsymbol{\Sigma} = C_i + C_j$ ; shared data or theoretical inputs introduce a cross term  $C_{ij} \simeq \rho C_{\text{common}}$ .

## B. COVARIANCE CONSTRUCTION AND REGULARIZATION

For Hessian ensembles (CT18, MSHT20), we use the symmetric prescription

$$\Delta f^2 = \frac{1}{4} \sum_{k=1}^{N_{\text{eig}}} (f_k^+ - f_k^-)^2, \quad (2)$$

and for Monte-Carlo ensembles (NNPDF) we take  $C = \langle \delta f \delta f^\top \rangle$  with  $\delta f = f^{(r)} - \langle f \rangle$ . A small Tikhonov regularization  $\lambda I$  with  $\lambda = 10^{-6} \times \text{median}(\text{diag } C)$  ensures numerical stability of  $\Sigma^{-1}$  on fine grids. All matrices are whitened and inverted via a Cholesky decomposition.

## C. LOCAL DIAGNOSTICS AND JEFFREYS DIVERGENCE

The local significance is defined by

$$T^2(x, Q) = \frac{(\mu_i - \mu_j)^2}{\sigma_i^2 + \sigma_j^2 - 2\sigma_{ij}}, \quad (3)$$

which approximately follows a  $\chi_k^2$  distribution. The symmetrized Kullback–Leibler (Jeffreys) divergence is given by

$$D_{\text{KL}}(i||j) = \frac{1}{2} \left[ \text{Tr}(C_j^{-1} C_i) + (\mu_j - \mu_i)^\top C_j^{-1} (\mu_j - \mu_i) - k + \ln \frac{\det C_j}{\det C_i} \right], \quad (4)$$

$$J(i, j) = \frac{1}{2} [D_{\text{KL}}(i||j) + D_{\text{KL}}(j||i)]. \quad (5)$$

## D. GRID AND PARAMETER SCANS

The  $(x, Q)$  grid spans  $x \in [10^{-6}, 10^{-2}]$  and  $Q \in [5, 500]$  GeV with logarithmic spacing. Variations over grid resolution,  $\rho$ , and  $\lambda$  define the systematic uncertainty bands shown in Fig. 3 of the main Letter.

## E. NUMERICAL RESOURCES

All calculations were performed using `LHAPDF6.5.3`, `APFEL` (NNLO FONLL-C scheme), and `MadGraph5_aMC@NLO`. Representative input cards and Python scripts for grid evaluation are included in the ancillary directory.
